# Supplementary material for: PyCDFT: A Python package for constrained density functional theory
Source: arXiv:2005.08021 ancillary file (2020-05-16)
Supplement: Supplementary file 1 [file jcc-supplementary.pdf]

# Supplementary Information for PyCDFT: A Python package for constrained density functional theory

He Ma[*,†], Wennie Wang[‡], Siyoung Kim[‡], Man-Hin Cheng[‡,§], Marco Govoni[†,‡], Giulia Galli[*,†,‡]

Submitted to Journal of Computational Chemistry

[*]Department of Chemistry, University of Chicago, Chicago, Illinois 60637, United States
[†]Materials Science Division and Center for Molecular Engineering, Argonne National Laboratory, Lemont, Illinois 60439, USA
[‡]Pritzker School of Molecular Engineering, University of Chicago, Chicago, Illinois 60637, United States
[§]Current Address: Department of Physics, ETH Zurich, 8093 Zurich, Switzerland

# S1 Calculated electronic couplings for the HAB18 dataset

Below we present calculated electronic couplings for the HAB18 dataset, as obtained by `PyCDFT`(Qbox), CP2K, CPMD, and QE, corresponding to the values shown in Fig. 6 in the main text.

Table S1: Diabatic electronic couplings $H_{ab}$ (in meV) and the coupling decay constant $\beta$ (in 1/Å) for the HAB18 data set. CPMD values are taken from Ref. 1, and italicized CPMD values are taken from Ref. 2; QE (Quantum Espresso) values are taken from Ref. 3.

| | Dist. (Å) | PyCDFT(Qbox) | CP2K | CPMD | QE |
|---|---|---|---|---|---|
| anthracene | 3.5 | 607.58 | 602.09 | *637.00* | 651.07 |
| | 4.0 | 294.91 | 286.61 | *324.50* | 329.15 |
| | 4.5 | 139.32 | 134.88 | *169.40* | 171.49 |
| | 5.0 | 71.37 | 58.34 | *87.90* | 91.60 |
| | $\beta$ | 2.904 | 3.008 | *2.64* | 2.618 |
| benzene | 3.5 | 641.21 | 633.08 | 647.80 | — |
| | 4.0 | 317.09 | 306.80 | 321.70 | — |
| | 4.5 | 155.95 | 142.59 | 155.60 | — |
| | 5.0 | 74.40 | 63.84 | 73.80 | — |
| | $\beta$ | 2.834 | 2.966 | 2.896 | — |
| cyclopentadiene | 3.5 | 702.38 | 690.49 | 702.10 | 699.45 |
| | 4.0 | 343.86 | 327.38 | 346.40 | 335.82 |
| | 4.5 | 168.04 | 152.11 | 167.40 | 159.32 |
| | 5.0 | 80.56 | 68.90 | 80.90 | 75.03 |
| | $\beta$ | 2.865 | 3.019 | 2.886 | 2.989 |
| cyclopropene | 3.5 | 814.35 | 796.12 | 816.10 | 810.11 |
| | 4.0 | 366.92 | 347.41 | 369.60 | 358.90 |
| | 4.5 | 164.25 | 151.54 | 164.80 | 157.57 |
| | 5.0 | 72.78 | 67.77 | 73.90 | 69.42 |
| | $\beta$ | 3.199 | 3.311 | 3.201 | 3.283 |
| ethylene | 3.5 | 616.44 | 601.10 | 621.50 | 611.67 |
| | 4.0 | 312.77 | 299.43 | 314.80 | 306.29 |
| | 4.5 | 159.19 | 149.53 | 158.30 | 153.01 |
| | 5.0 | 80.02 | 74.80 | 78.40 | — |
| | $\beta$ | 2.713 | 2.783 | 2.761 | 2.669 |

Table S1: Continued.

| | Dist. (Å) | PyCDFT(Qbox) | CP2K | CPMD | QE |
|---|---|---|---|---|---|
| furane | 3.5 | 599.19 | 585.70 | 598.20 | 594.68 |
| | 4.0 | 292.02 | 278.70 | 292.50 | 285.25 |
| | 4.5 | 142.69 | 129.97 | 141.00 | 136.33 |
| | 5.0 | 68.45 | 59.10 | 67.00 | 65.36 |
| | $\beta$ | 2.876 | 3.005 | 2.919 | 3.001 |
| imidazole | 3.5 | 590.97 | 574.87 | 590.10 | 586.23 |
| | 4.0 | 285.84 | 271.47 | 286.30 | 278.88 |
| | 4.5 | 138.53 | 125.07 | 136.80 | 132.22 |
| | 5.0 | 66.11 | 60.85 | 64.30 | 63.01 |
| | $\beta$ | 2.907 | 3.019 | 2.953 | 3.029 |
| pentacene | 3.5 | 595.38 | 597.25 | *618.30* | 645.97 |
| | 4.0 | 280.42 | 267.81 | *303.00* | 309.60 |
| | 4.5 | — | 124.74 | *154.00* | 156.82 |
| | 5.0 | 65.22 | 56.38 | *77.70* | 80.19 |
| | $\beta$ | 2.944 | 3.166 | *2.76* | 2.706 |
| perfluoroanthracene | 3.5 | 410.62 | 411.72 | *479.60* | 479.46 |
| | 4.0 | 180.56 | 178.48 | *227.20* | 219.90 |
| | 4.5 | 73.19 | 70.01 | *107.90* | 99.96 |
| | 5.0 | 35.24 | 29.48 | *49.60* | 45.01 |
| | $\beta$ | 3.345 | 3.444 | *3.02* | 3.158 |
| perylene | 3.5 | 595.38 | 583.35 | *553.70* | 654.05 |
| | 4.0 | 280.42 | 272.54 | *324.50* | 332.83 |
| | 4.5 | 137.63 | 124.72 | *174.00* | 178.72 |
| | 5.0 | 65.22 | 55.24 | *94.40* | 100.26 |
| | $\beta$ | 2.964 | 3.08 | *2.54* | 2.503 |

Table S1: Continued.

| | Dist. (Å) | PyCDFT(Qbox) | CP2K | CPMD | QE |
|---|---|---|---|---|---|
| phenol | 3.5 | 560.23 | 546.87 | 557.30 | 557.29 |
| | 4.0 | 271.43 | 257.89 | 271.30 | 264.94 |
| | 4.5 | 130.74 | 115.91 | 129.70 | 123.52 |
| | 5.0 | 61.14 | 54.07 | 58.90 | 56.87 |
| | $\beta$ | 2.915 | 3.06115 | 2.996 | 3.112 |
| porphin | 3.5 | 569.86 | 557.49 | *577.70* | 590.25 |
| | 4.0 | 273.96 | 267.26 | *285.00* | 288.54 |
| | 4.5 | 139.76 | 128.95 | *146.60* | 146.85 |
| | 5.0 | 76.90 | 58.59 | *74.70* | 76.17 |
| | $\beta$ | 2.815 | 2.949 | *2.72* | 2.729 |
| pyrrole | 3.5 | 632.18 | 618.01 | 629.80 | 629.02 |
| | 4.0 | 315.00 | 300.62 | 314.80 | 309.13 |
| | 4.5 | 157.49 | 143.35 | 155.50 | 151.59 |
| | 5.0 | 77.43 | 66.60 | 75.70 | 74.56 |
| | $\beta$ | 2.786 | 2.9184 | 2.82 | 2.905 |
| tetracene | 3.5 | 597.11 | 586.20 | *628.80* | 644.67 |
| | 4.0 | 285.50 | 276.77 | *313.10* | 318.79 |
| | 4.5 | 140.46 | 128.43 | *160.80* | 163.00 |
| | 5.0 | 69.20 | 58.89 | *81.50* | 84.36 |
| | $\beta$ | 2.910 | 3.028 | *2.72* | 2.712 |
| thiophene | 3.5 | 679.76 | 660.65 | 669.90 | 676.13 |
| | 4.0 | 334.35 | 314.05 | 332.30 | 328.24 |
| | 4.5 | 164.33 | 146.85 | 162.40 | 158.10 |
| | 5.0 | 78.58 | 66.07 | 77.40 | 75.61 |
| | $\beta$ | 2.847 | 3.007 | 2.881 | 2.988 |

Tables S2 and S3 show additional statistical metrics for measuring variation of `PyCDFT` with CP2K, CPMD, and QE implementations.

Table S2: Mean error (ME, meV), mean absolute error (MAE, meV), root-mean-square-deviation (RMSD, meV), and mean absolute percent error (MAPE, %) of the electron coupling $H_{ab}$ for the HAB18 dataset comparing PyCDFT(Qbox) with CP2K, CPMD, and QE.

| $H_{ab}$ | CP2K | CPMD | QE |
|---|---|---|---|
| ME (meV) | 10.98 | -8.68 | -10.46 |
| MAE (meV) | 11.09 | 11.38 | 16.58 |
| RMSD (meV) | 11.99 | 19.03 | 24.11 |
| MAPE (%) | 7.69 | 5.74 | 7.83 |

Table S3: Mean error (ME, 1/Å), mean absolute error (MAE, 1/Å), root-mean-square-deviation (RMSD, 1/Å), and mean absolute percent error (MAPE, %) of the decay constant $\beta$ for the HAB18 dataset comparing PyCDFT(Qbox) with CP2K, CPMD, and QE.

| $\beta$ | CP2K | CPMD | QE |
|---|---|---|---|
| ME (1/Å) | -0.13 | -0.07 | 0.04 |
| MAE (1/Å) | 0.13 | 0.12 | 0.17 |
| RMSD (1/Å) | 0.13 | 0.17 | 0.20 |
| MAPE (%) | 4.24 | 4.49 | 6.16 |

# S2 Numerical stability for the calculation of Hirshfeld weight functions

In the calculation of Hirshfeld weight functions in Eq. 3 and Eq. 4, we adopted an adjustable numerical cutoff `eps` for the electron density in the denominator to avoid numerical instabilities. When the electron density is smaller than `eps`, the weight function is set to zero. We use a default value of $10^{-6}$ for `eps`, which we found to yield accurate electronic couplings in all cases considered here. In Fig. S1, we show a benchmark of `eps` parameter for the CDFT calculation of $He_2^+$.

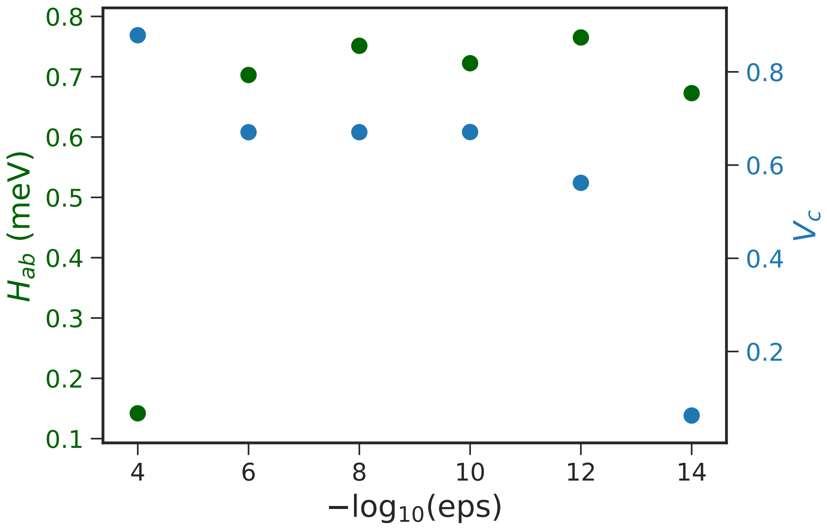


Figure S1: Effect of the chosen `eps` parameter (see text) on the computed electronic coupling $H_{ab}$ of $He_2^+$ with a bond length of 5.0 Å; the corresponding constraint potential $V_c$ is also shown. Too large `eps` values lead to over-truncation of the electron density and hence to an underestimation of the electronic coupling. Too small `eps` values give rise to numerical instabilities due to the small denominators in the evaluation of weight functions. An `eps` value between $10^{-6}$ and $10^{-10}$ yields reasonable results for the electronic coupling.

# S3 Verification of force evaluations

In `PyCDFT` we evaluate constraint forces using the analytical expression shown in Eq. 6. In Fig. S2 we show that the forces evaluated through Eq. 6 is in good agreement with numerical finite difference calculations.

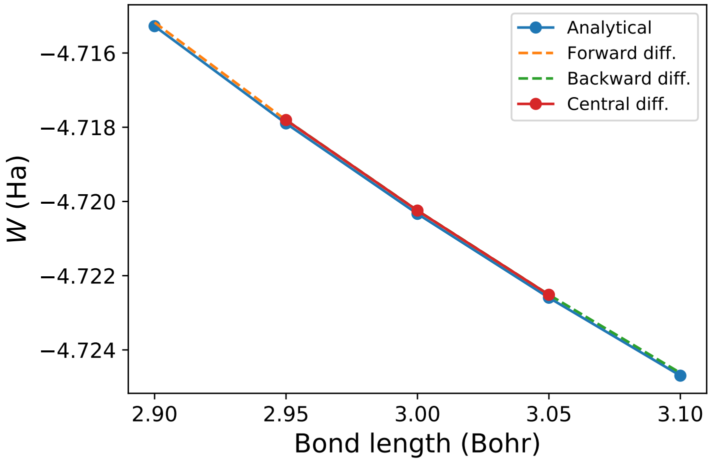


Figure S2: Comparison of the analytical forces evaluated using Eq. 6 with forces computed by numerical finite differences for $He_2^+$ at various bond lengths.

# References

[1] A. Kubas, F. Hoffmann, A. Heck, H. Oberhofer, M. Elstner, and J. Blumberger, The Journal of Chemical Physics **140**, 104105 (2014), ISSN 0021-9606, 1089-7690.

[2] A. Kubas, F. Gajdos, A. Heck, H. Oberhofer, M. Elstner, and J. Blumberger, Physical Chemistry Chemical Physics **17**, 14342 (2015), ISSN 1463-9076, 1463-9084.

[3] M. B. Goldey, N. P. Brawand, M. Vörös, and G. Galli, Journal of Chemical Theory and Computation **13**, 2581 (2017), ISSN 1549-9618, 1549-9626.
